# Supplementary material for: Role of interaction anisotropy in polymer cononsolvency: insights from the Flory-Huggins-Potts framework
Source: arXiv:2506.06960 source file (2025-09-27)
Supplement: Supplementary file 2 [file packages_supp.tex]

\setlength{\oddsidemargin}{0in}
\setlength{\textwidth}{6.5in}
\setlength{\topmargin}{-0.5in}
\setlength{\textheight}{9in}

\usepackage{amsmath,amssymb, mathtools}
\usepackage{titlesec}
\titleformat{\section}
  {\normalfont\fontsize{14}{15}\bfseries}{\thesection}{1em}{}
\titleformat*{\subsection}{\small\bfseries}
\titleformat*{\subsubsection}{\small\bfseries}

\usepackage{graphicx}
\usepackage{dcolumn}
\usepackage{bm}
\usepackage{upgreek}
\usepackage[numbers,super,comma,sort&compress]{natbib}
\usepackage{lipsum}  
\usepackage{tabularx}
\usepackage{booktabs}
\usepackage{enumitem}
\usepackage{setspace}
\usepackage{array}
\usepackage[makeroom]{cancel}
\usepackage{empheq}
\newcommand\widecolourbox[1]{{\setlength\fboxrule{1pt}\setlength\fboxsep{8pt}\fcolorbox{black}{white}{\enspace#1\enspace }}}

\newcommand{\smallerSection}[1]{\titleformat{\section}{\large\bfseries\filcenter}{\thesection}{1em}{\MakeUppercase{#1}}}
\newcommand{\mySection}[1]{\section*{\sffamily \large {#1}}}
\newcommand{\mySubSection}[1]{\section*{\sffamily \normalsize {#1}}}

\DeclareRobustCommand*{\citen }[1]{
  \begingroup
    \romannumeral-`\x
    \setcitestyle{numbers} 
    \cite{#1} 
  \endgroup   
}
\usepackage{xcolor}


\usepackage[parfill]{parskip}

\usepackage{wasysym}
\usepackage[font=footnotesize]{caption}
\usepackage{float}
\usepackage{capt-of}
\usepackage{helvet}
\usepackage{enumitem}
\usepackage{relsize}
\usepackage{makecell}

\makeatletter
\newcommand*{\addFileDependency}[1]{
  \typeout{(#1)}
  \@addtofilelist{#1}
  \IfFileExists{#1}{}{\typeout{No file #1.}}
}
\makeatother
\newcommand*{\myexternaldocument}[1]{
    \externaldocument{#1}
    \addFileDependency{#1.tex}
    \addFileDependency{#1.aux}
}
